# Supplementary material for: Star formation history of the solar neighbourhood as told by Gaia
Source: arXiv:2011.05732 source file (2020-11-11)
Supplement: Supplementary file 1 [file A3_supporting_information.tex]

%\section{SUPPORTING INFORMATION}\label{bhmtab}

\setcounter{table}{1}    

\input{table_D1}
\input{table_D2}
\input{table_D3}

\setcounter{figure}{20}    

\input{figure_D3}
\input{figure_D1}
\input{figure_D2}
